# Supplementary material for: Habitat-Web: Learning Embodied Object-Search Strategies from Human Demonstrations at Scale
Source: arXiv:2204.03514 source file (2022-04-08)
Supplement: Supplementary file 1 [file cvpr_supplement.tex]

% % CVPR 2022 Paper Template
% % based on the CVPR template provided by Ming-Ming Cheng (https://github.com/MCG-NKU/CVPR_Template)
% % modified and extended by Stefan Roth (stefan.roth@NOSPAMtu-darmstadt.de)

% \documentclass[10pt,twocolumn,letterpaper]{article}
% \usepackage[review]{cvpr}
% \input{imports}

% %%%%%%%%% PAPER TYPE  - PLEASE UPDATE FOR FINAL VERSION
% % \usepackage[review]{cvpr}      % To produce the REVIEW version
% %\usepackage{cvpr}              % To produce the CAMERA-READY version
% %\usepackage[pagenumbers]{cvpr} % To force page numbers, e.g. for an arXiv version

% % Include other packages here, before hyperref.
% % \usepackage{graphicx}
% % \usepackage{amsmath}
% % \usepackage{amssymb}
% % \usepackage{booktabs}


% % It is strongly recommended to use hyperref, especially for the review version.
% % hyperref with option pagebackref eases the reviewers' job.
% % Please disable hyperref *only* if you encounter grave issues, e.g. with the
% % file validation for the camera-ready version.
% %
% % If you comment hyperref and then uncomment it, you should delete
% % (Or just hit 'q' on the first LaTeX run, let it finish, and you
% %  should be clear).
% % \usepackage[pagebackref,breaklinks,colorlinks]{hyperref}


% % Support for easy cross-referencing
% \usepackage[capitalize]{cleveref}
% \crefname{section}{Sec.}{Secs.}
% \Crefname{section}{Section}{Sections}
% \Crefname{table}{Table}{Tables}
% \crefname{table}{Tab.}{Tabs.}


% %%%%%%%%% PAPER ID  - PLEASE UPDATE
% \def\cvprPaperID{4844} % *** Enter the CVPR Paper ID here
% \def\confName{CVPR}
% \def\confYear{2022}


% \begin{document}

% %%%%%%%%% TITLE - PLEASE UPDATE
% %\title{Learning Embodied Visual Exploration from Humans}
% % \title{Emergence of Efficient Object-Search Behavior in Embodied Agents \\
% % from Large-Scale Imitation of Human Demonstrations}
% %\title{Emergence of Strategic Object-Search Behavior in Embodied Agents \\
% %from Large-Scale Human Imitation}
% %\title{\datasetname: Learning Embodied Object-Search Strategies from Humans}
% \title{Learning Embodied Object-Search Strategies from 50k Human Demonstrations (Supplementary Material)}

% \author{First Author\\
% Institution1\\
% Institution1 address\\
% {\tt\small firstauthor@i1.org}
% % For a paper whose authors are all at the same institution,
% % omit the following lines up until the closing ``}''.
% % Additional authors and addresses can be added with ``\and'',
% % just like the second author.
% % To save space, use either the email address or home page, not both
% \and
% Second Author\\
% Institution2\\
% First line of institution2 address\\
% {\tt\small secondauthor@i2.org}
% }
% \maketitle


% \input{sections/supplement/appendix}
% \input{sections/supplement/analysis_figure}

% \bibliographystyle{ieeetr}
% %\biboptions{sort&compress}
% \bibliography{strings,main}

% %%%%%%%%% REFERENCES
% % {\small
% % \bibliographystyle{ieee_fullname}
% % \bibliography{egbib}
% % }

% \end{document}
